# Supplementary material for: AIR: Adaptive Interleaved Reasoning with Code in MLLMs
Source: arXiv:2606.23678 source file (2026-06-22)
Supplement: Supplementary file 1 [file limitations.tex]

\section{Limitations}
